# Supplementary material for: On structure, family and parameter estimation of hierarchical Archimedean copulas
Source: arXiv:1611.09225 ancillary file (2016-11-18)
Supplement: Supplementary file 1 [file attachment.pdf]

# An attachment to “On structure, family and parameter estimation of hierarchical Archimedean copulas”

-

The experimental results for  $d \in \{5, 10\}$ <sup>1</sup>

J. Górecki<sup>1</sup>, M. Hofert<sup>2</sup> and M. Holeňa<sup>3</sup>

<sup>1</sup>) Department of Informatics, SBA in Karviná, Silesian University in Opava, Univerzitní náměstí 1934/3, 733 40 Karviná, Czech Republic

gorecki@opf.slu.cz

<sup>2</sup>) Department of Statistics and Actuarial Science, University of Waterloo, 200 University Avenue West, Waterloo, ON, Canada

marius.hofert@uwaterloo.ca

<sup>3</sup>) Institute of Computer Science, Academy of Sciences of the Czech Republic, Pod vodárenskou věží 271/2, 182 07 Praha, Czech Republic

martin@cs.cas.cz

This attachment shows for  $d \in \{5, 10\}$  the results of the experiments described in the work “On structure, family and parameter estimation of hierarchical Archimedean copulas”. Section 1 shows the results of the estimators under the assumption that the underlying families are known (the  $\mathcal{F}$ -known scenario) and Section 2 shows the results of the estimators under the assumption that the underlying families are unknown (the  $\mathcal{F}$ -unknown scenario).

## 1 The $\mathcal{F}$ -known scenario

For each evaluation criterion,  $d \in \{5, 10\}$  and attitude, one figure is shown, and each figure is designed in the same way as in the main work, with only one change that the corresponding aggregated evaluation is added at the bottom of the figure. Also note that the aggregated evaluation is not included for the rejection rate. Also note that the optimistic case is not shown for the rejection rate.

---

<sup>1</sup>This attachment has been submitted to Journal of Statistical Computation and Simulation.

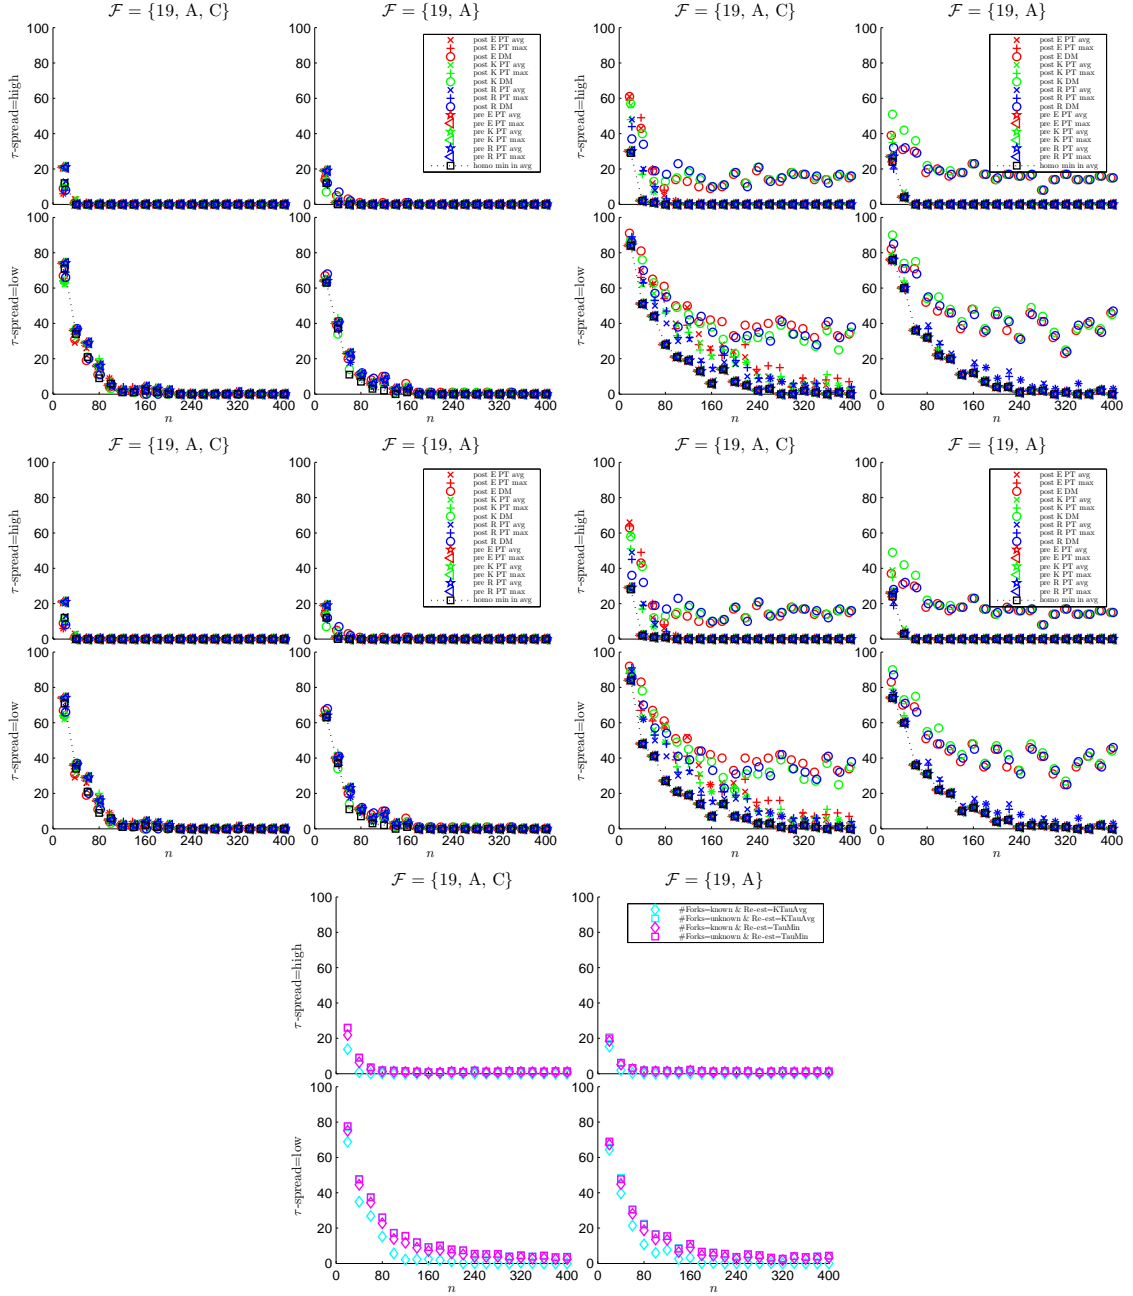

Figure 1: False structure ratio (in %) \*\*\* d=5 \*\*\* optimistic

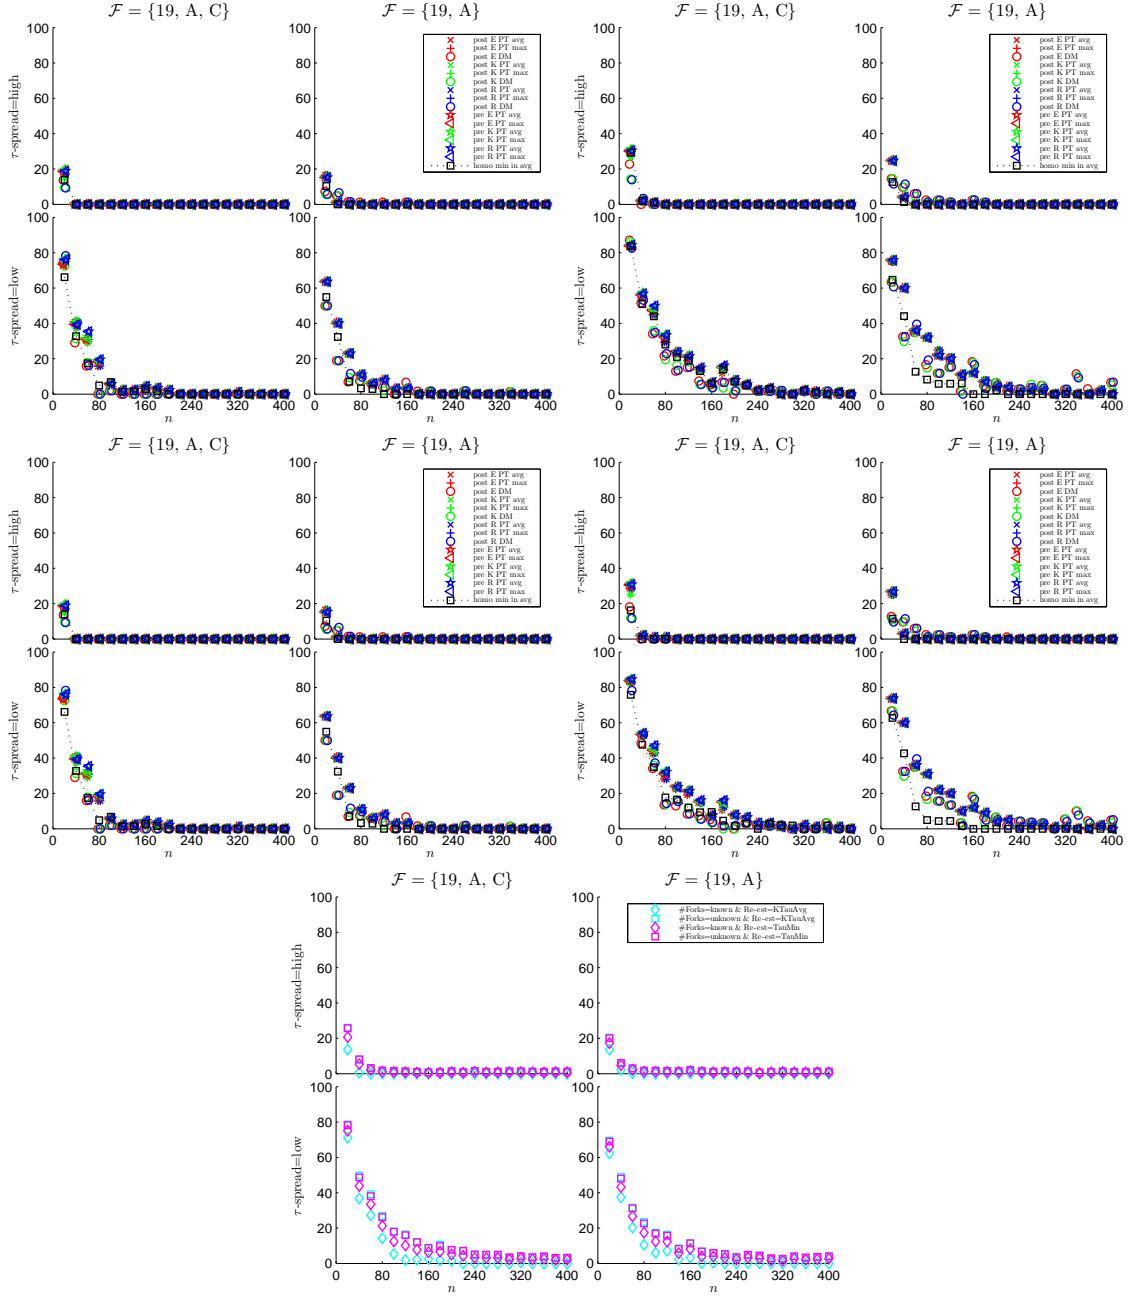

Figure 2: False structure ratio (in %) \*\*\* d=5 \*\*\* pessimistic

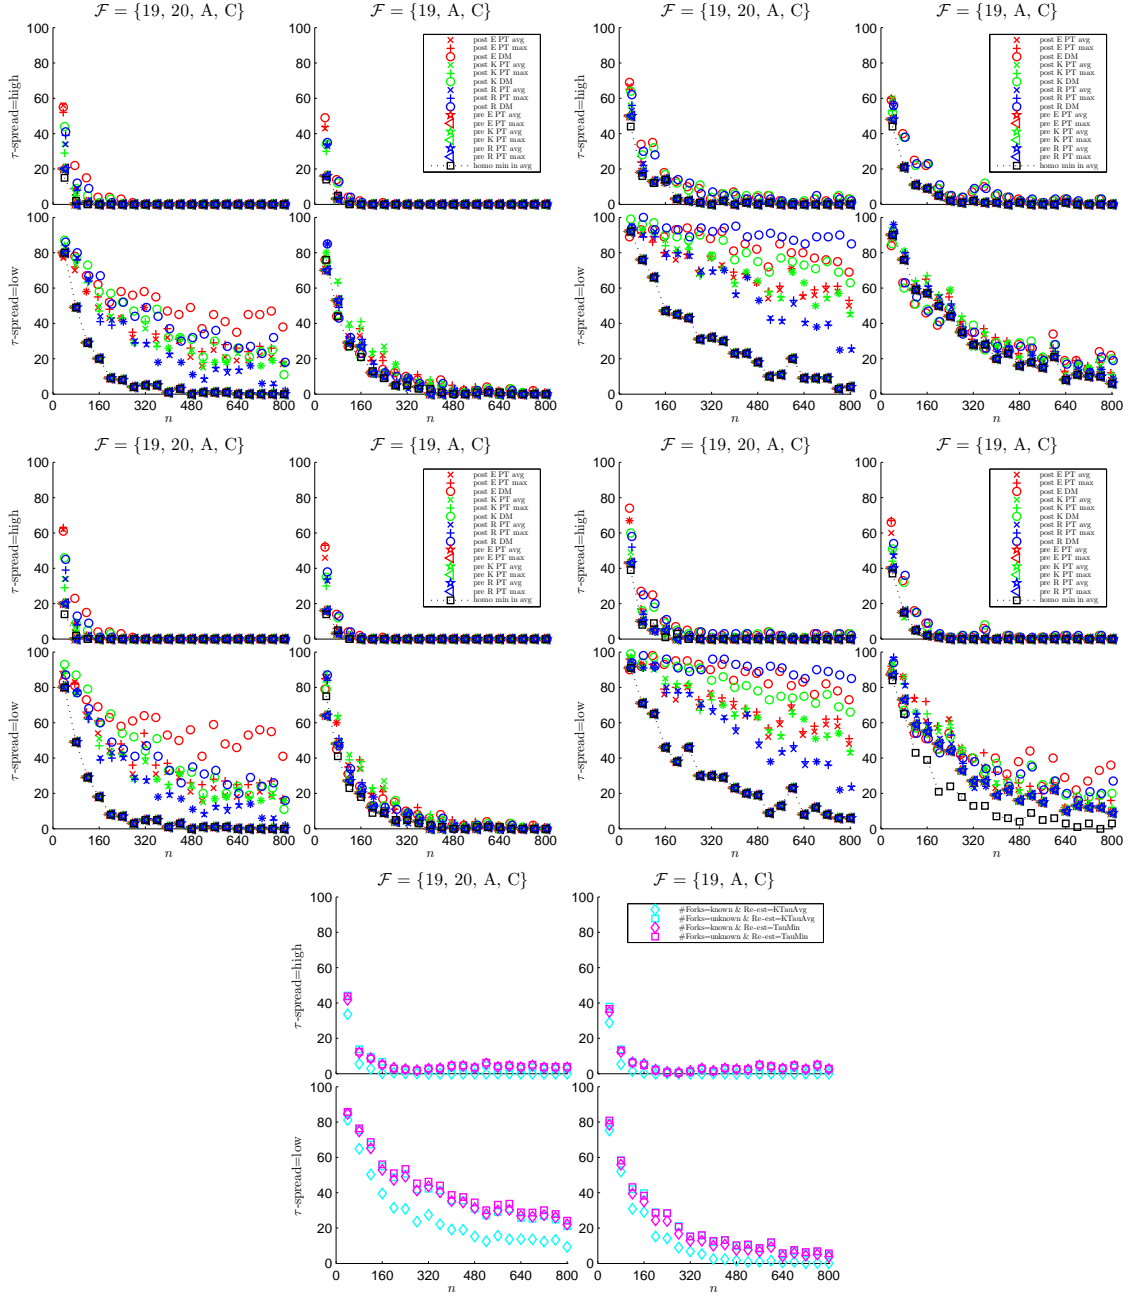

Figure 3: False structure ratio (in %) \*\*\* d=10 \*\*\* optimistic



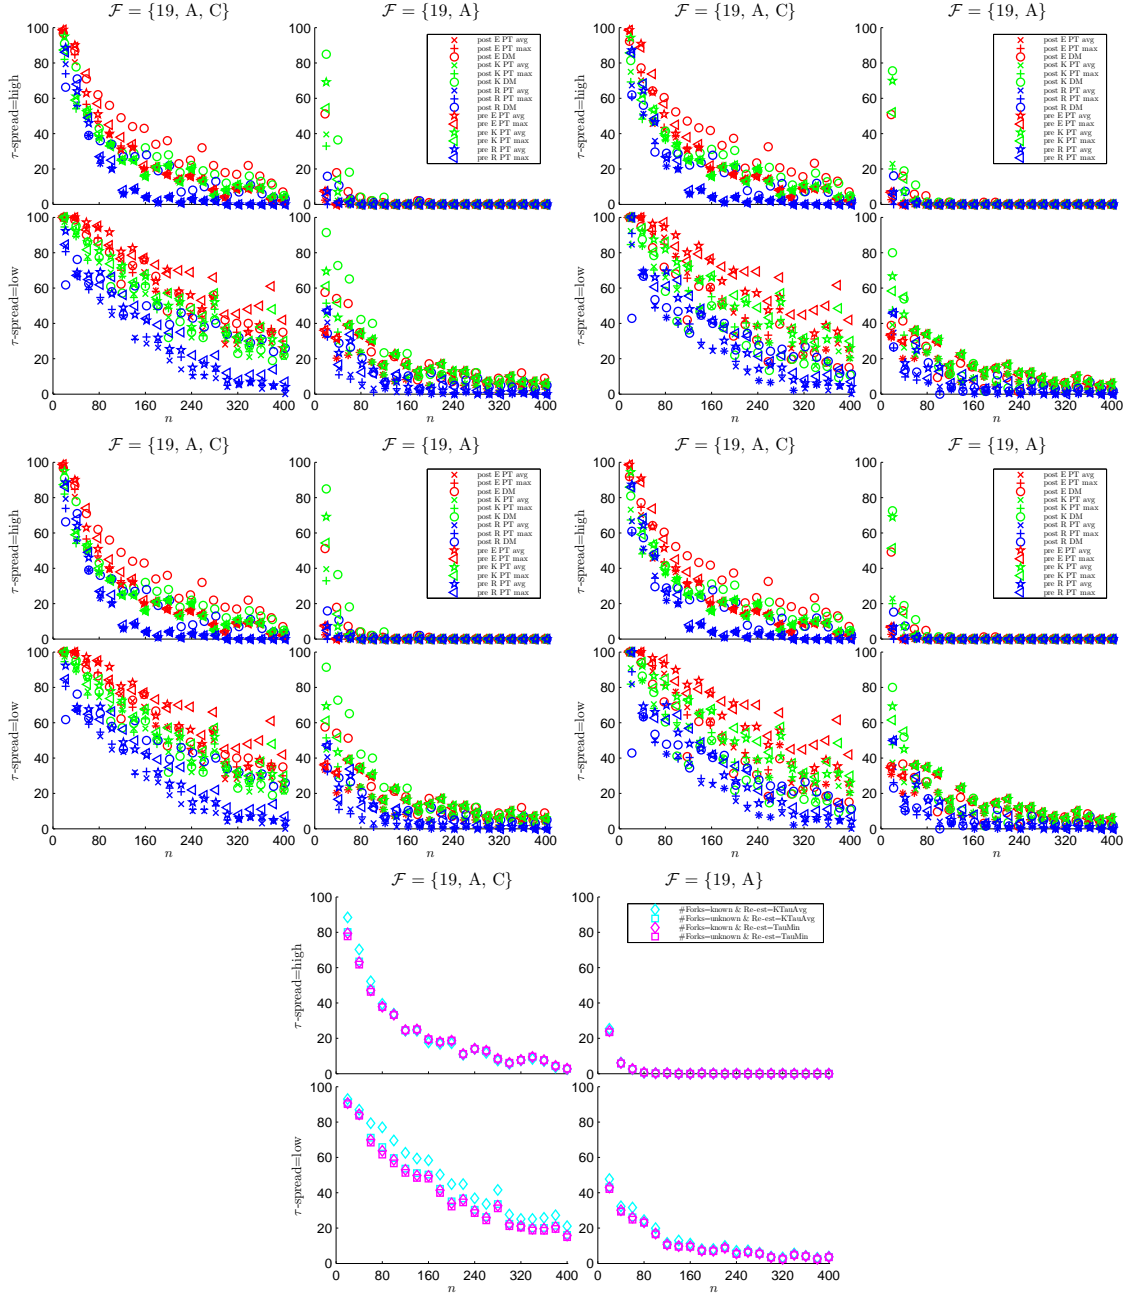

Figure 5: False families ratio (in %) \*\*\* d=5 \*\*\* optimistic

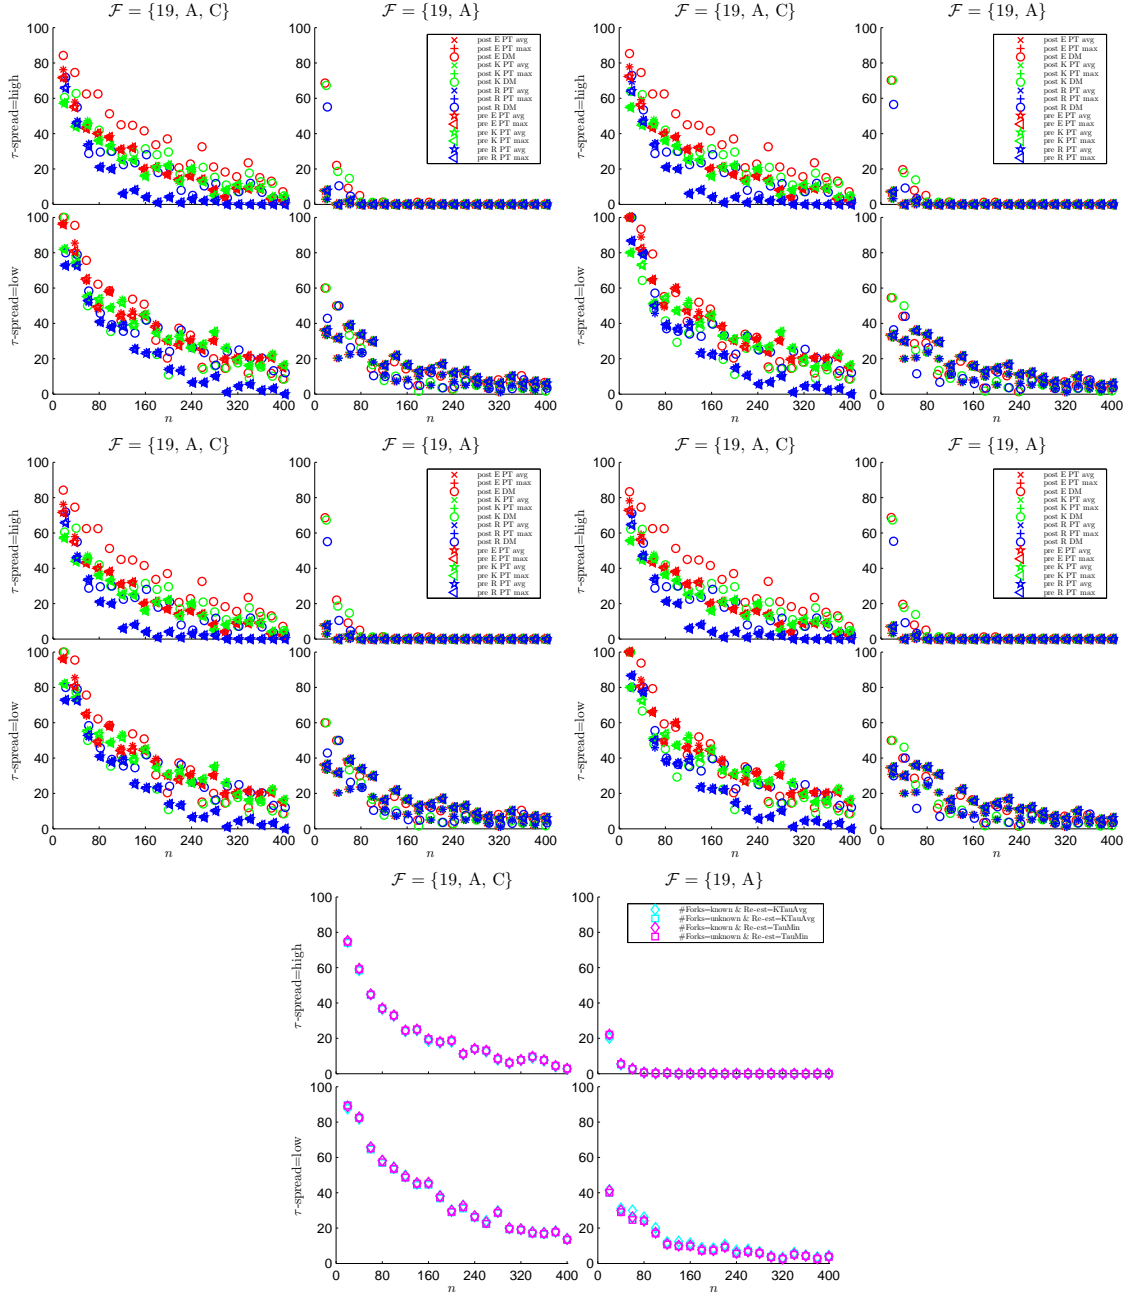

Figure 6: False families ratio (in %) \*\*\* d=5 \*\*\* pessimistic

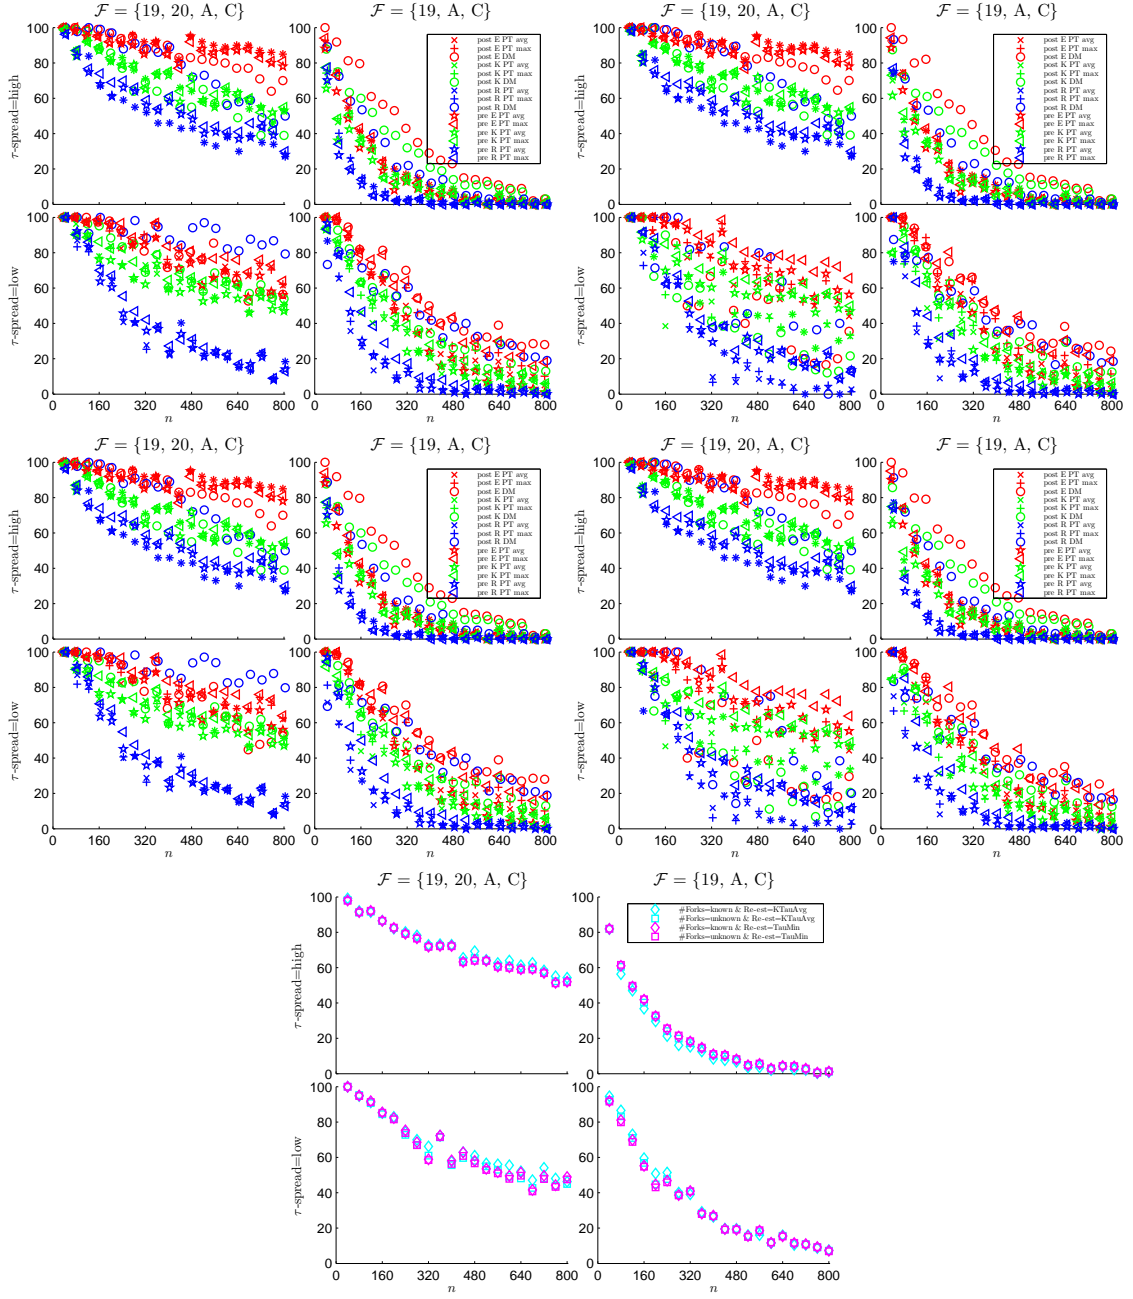

Figure 7: False families ratio (in %) \*\*\*  $d=10$  \*\*\* optimistic

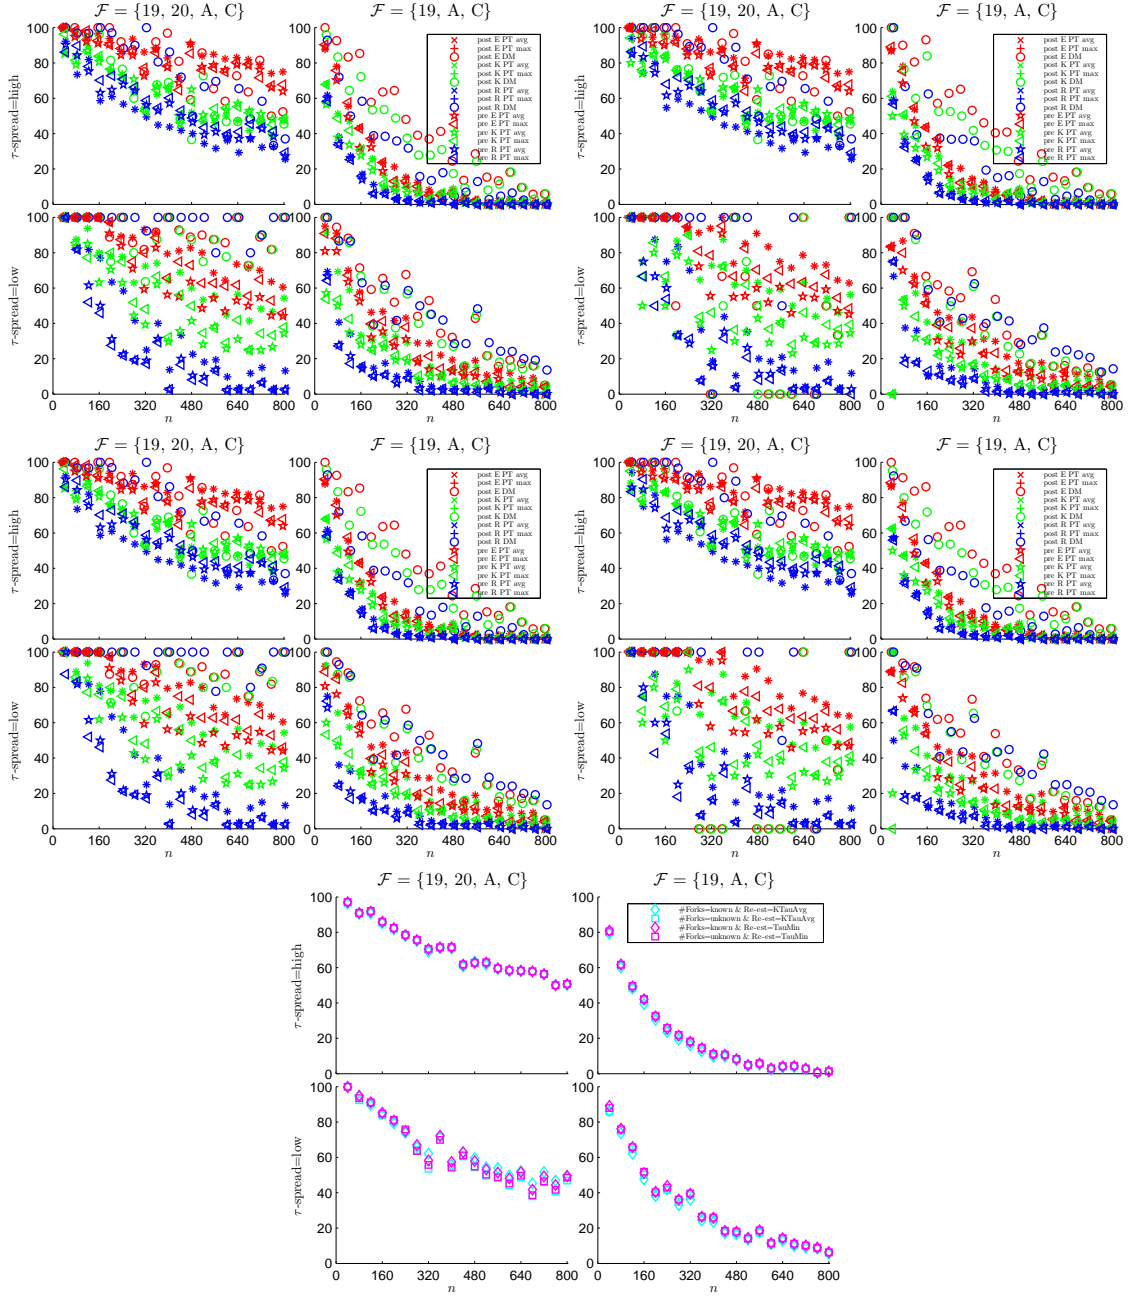

Figure 8: False families ratio (in %) \*\*\* d=10 \*\*\* pessimistic



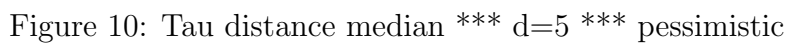

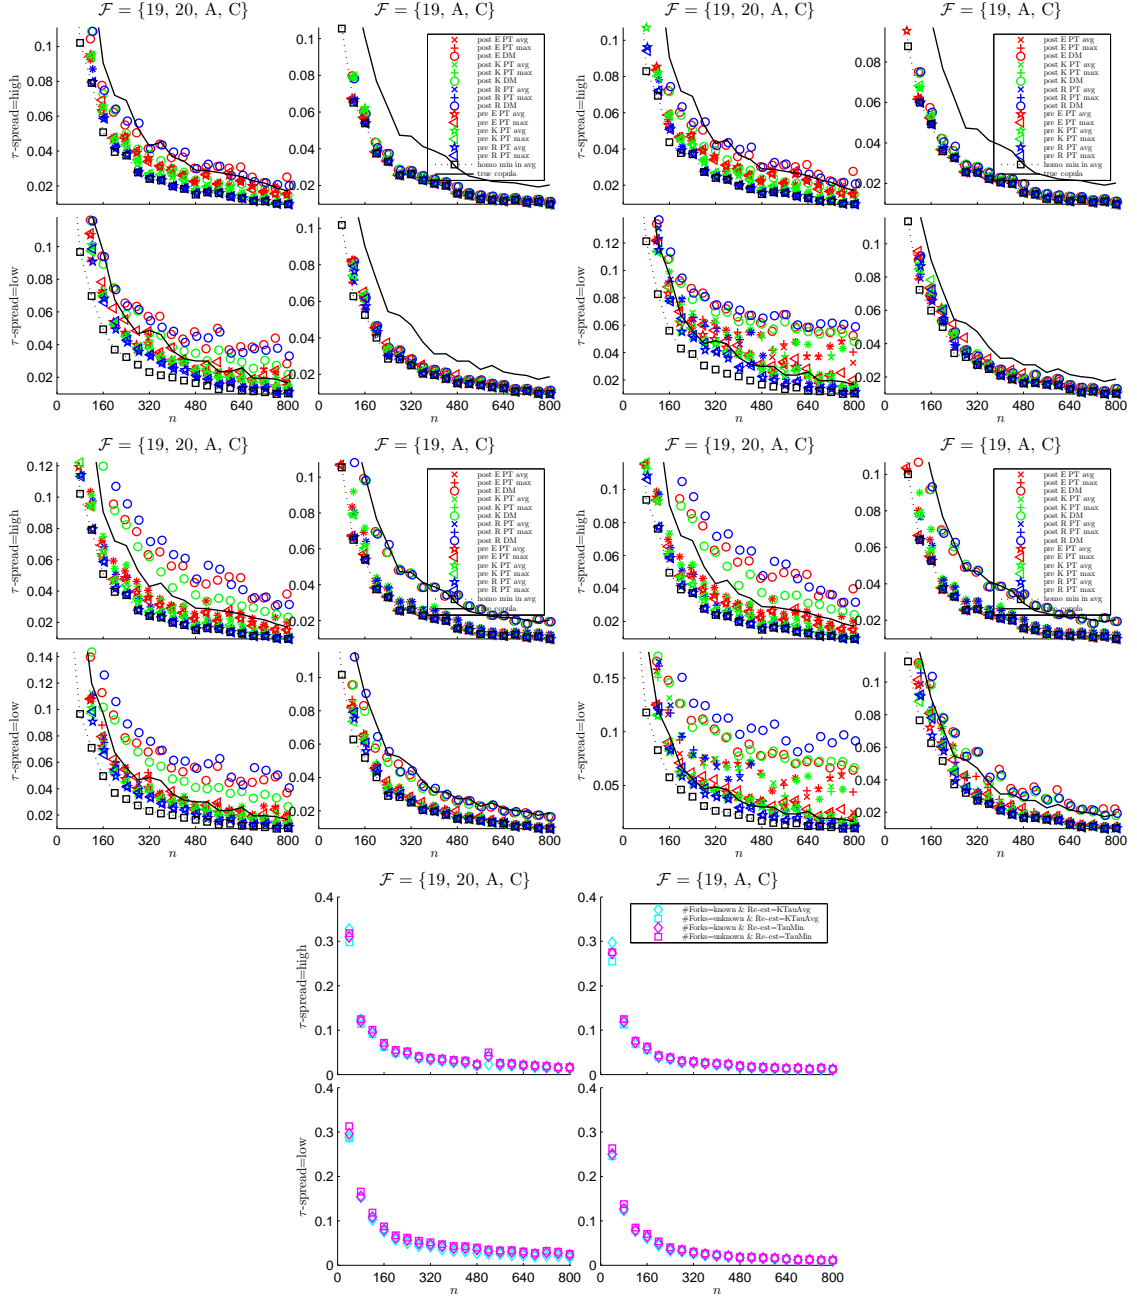

Figure 11: Tau distance median \*\*\* d=10 \*\*\* optimistic

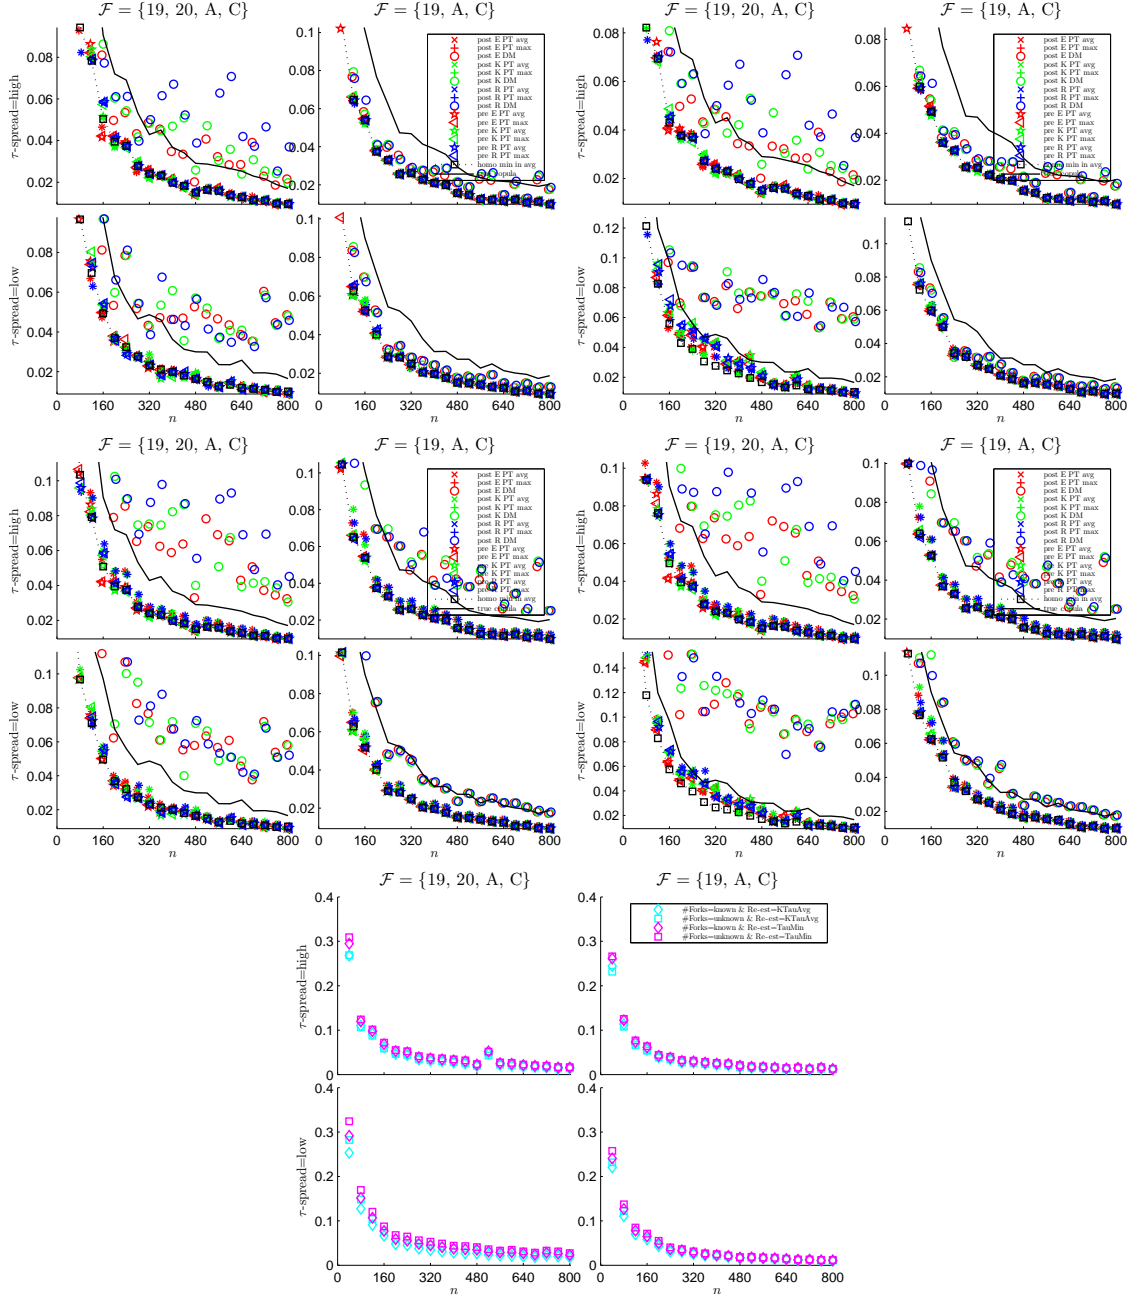

Figure 12: Tau distance median \*\*\*  $d=10$  \*\*\* pessimistic

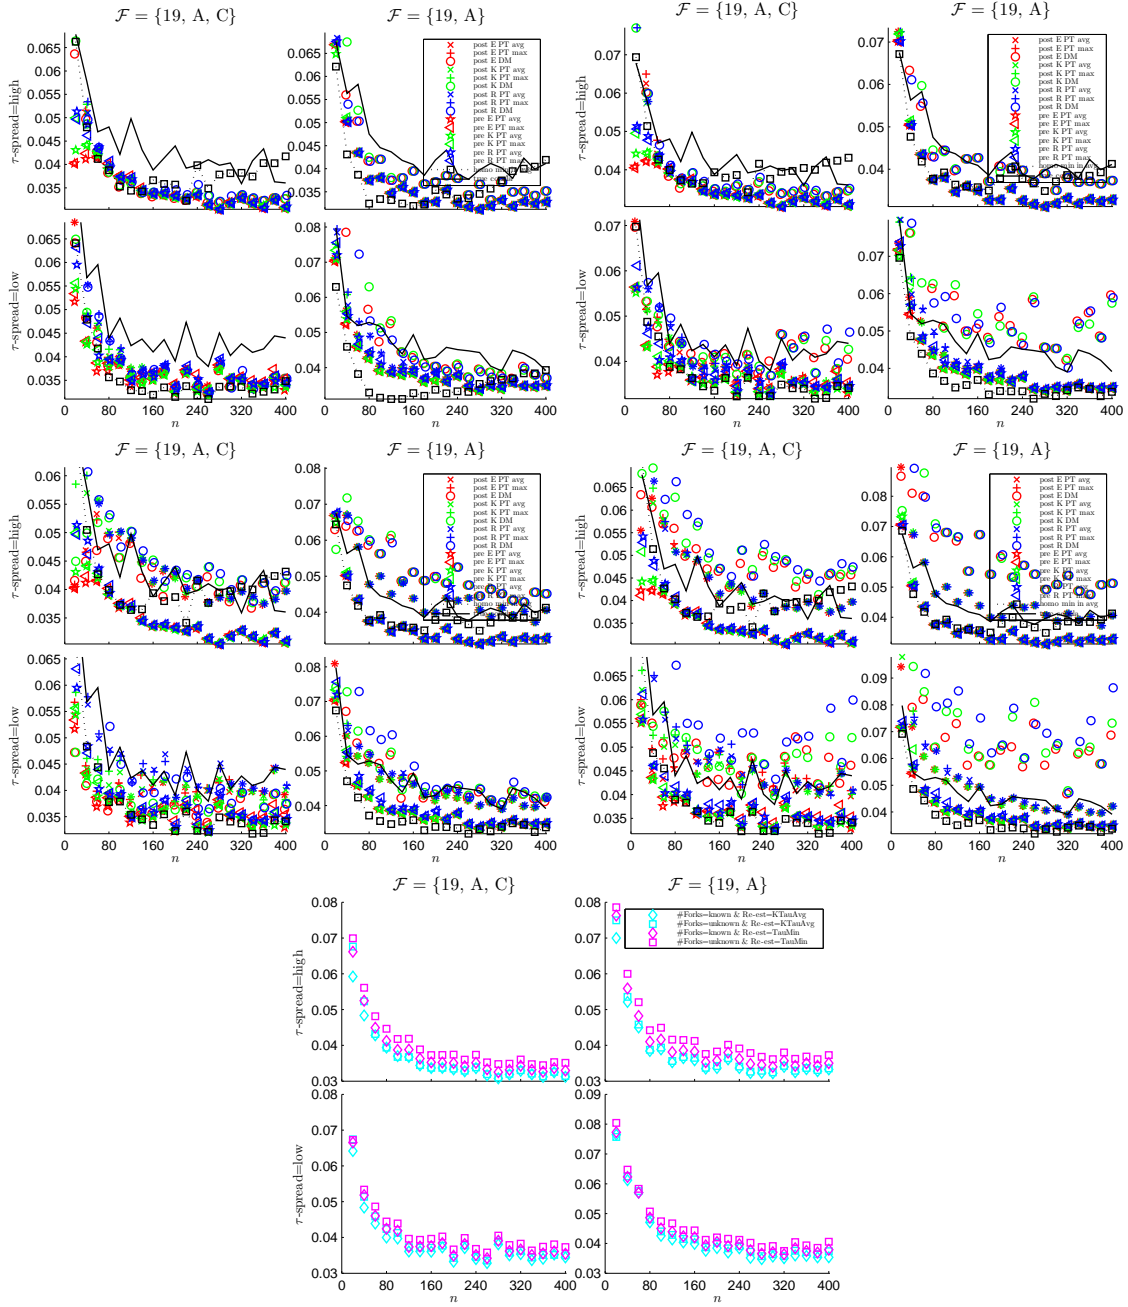

Figure 13: GoF median \*\*\*  $d=5$  \*\*\* optimistic

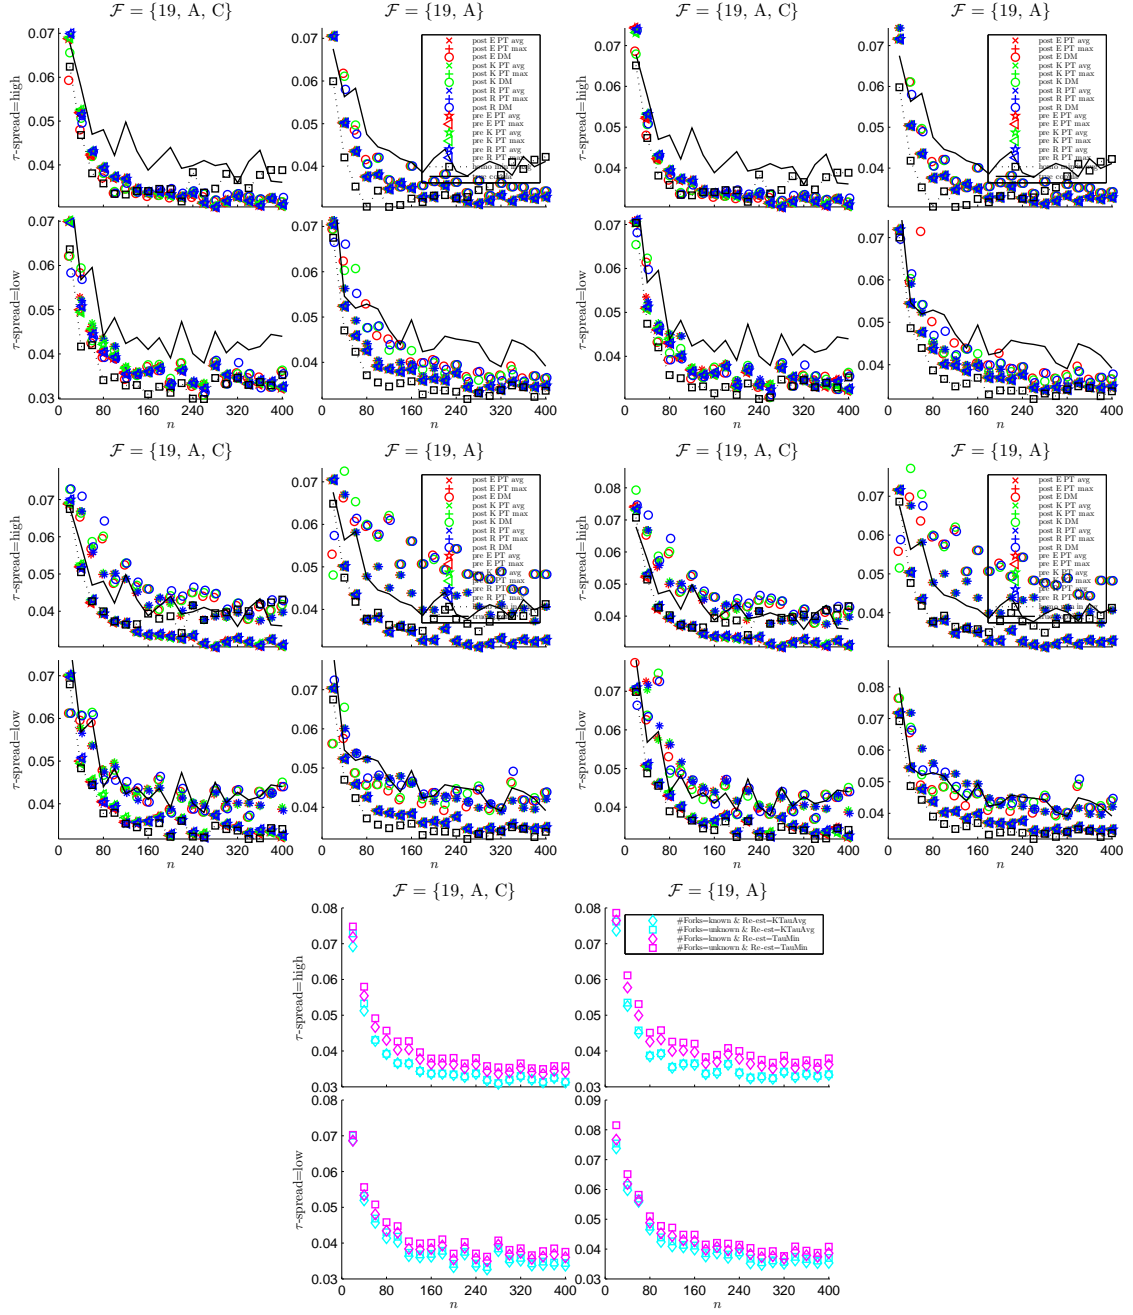

Figure 14: GoF median \*\*\* d=5 \*\*\* pessimistic

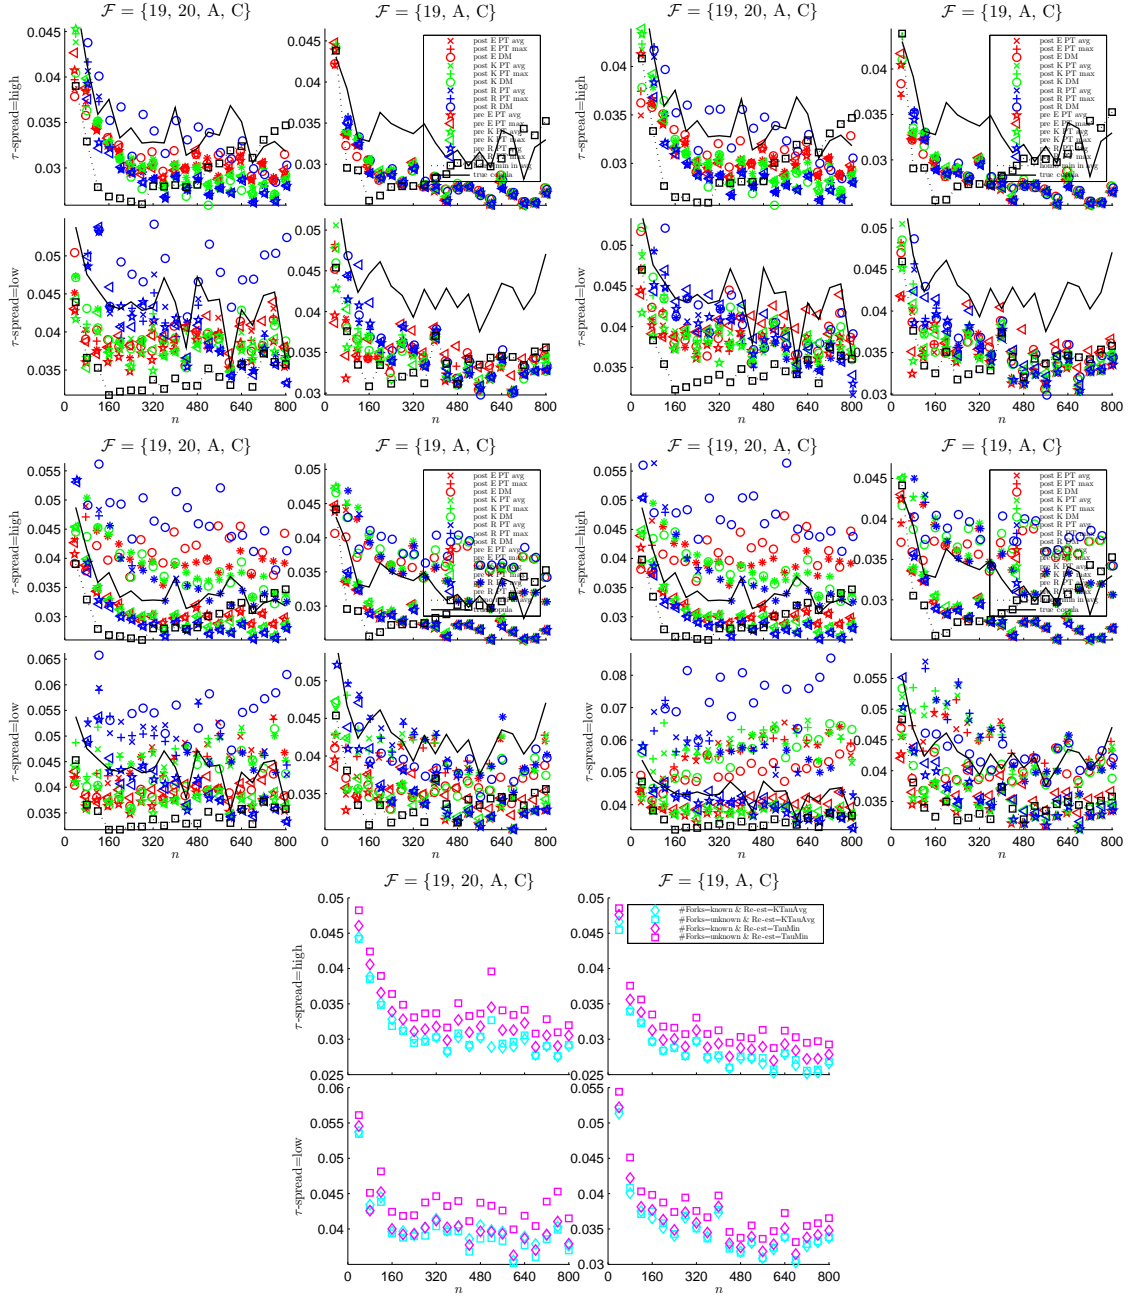

Figure 15: GoF median \*\*\*  $d=10$  \*\*\* optimistic

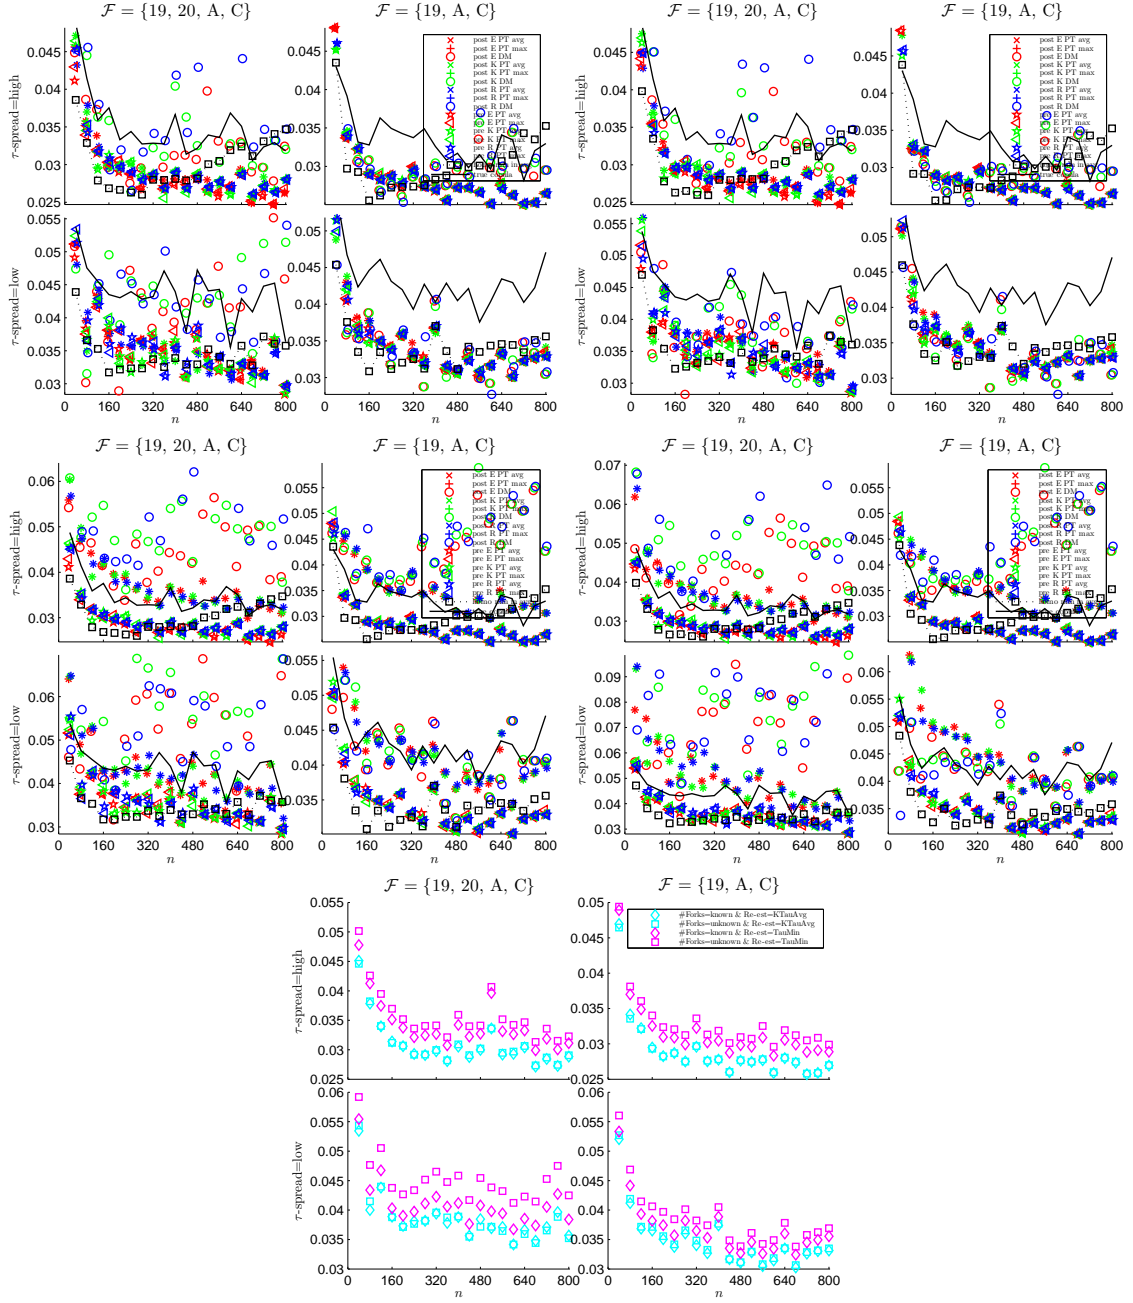

Figure 16: GoF median \*\*\*  $d=10$  \*\*\* pessimistic

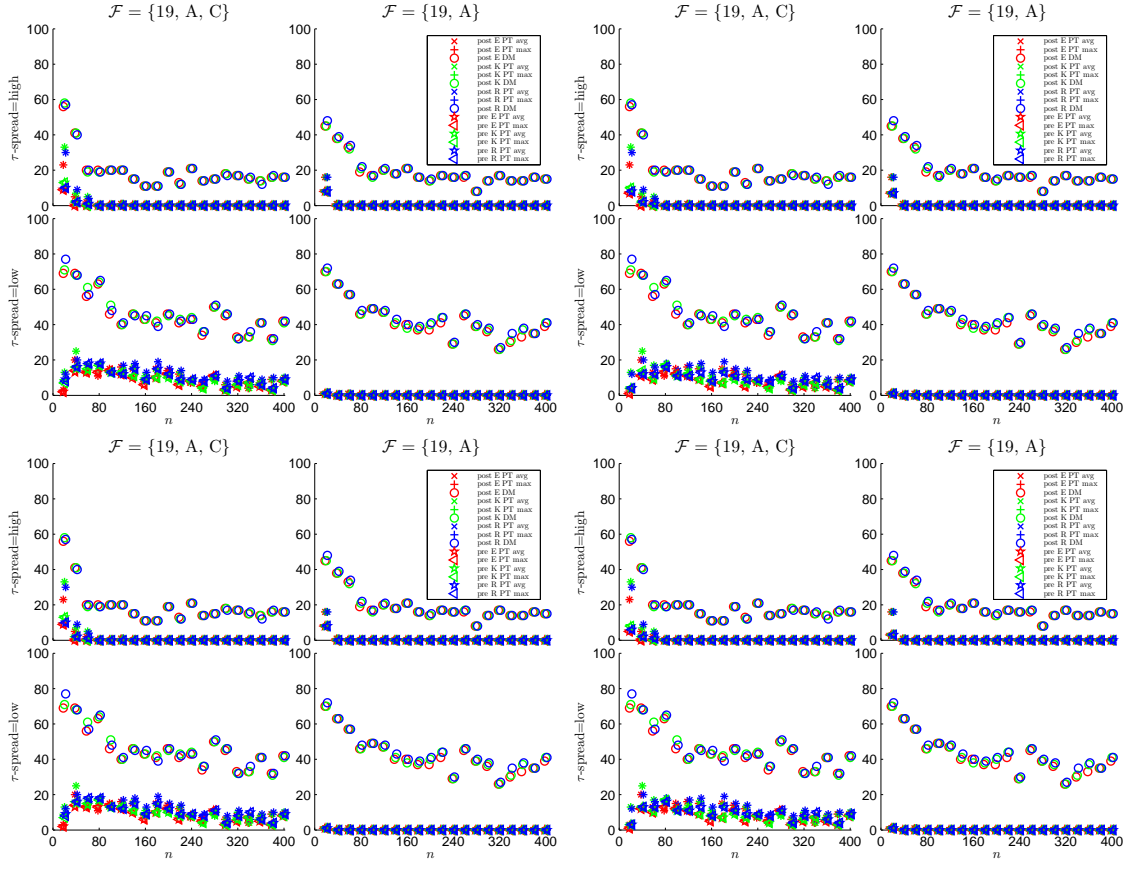

Figure 17: Rejection rate \*\*\* d=5 \*\*\* pessimistic

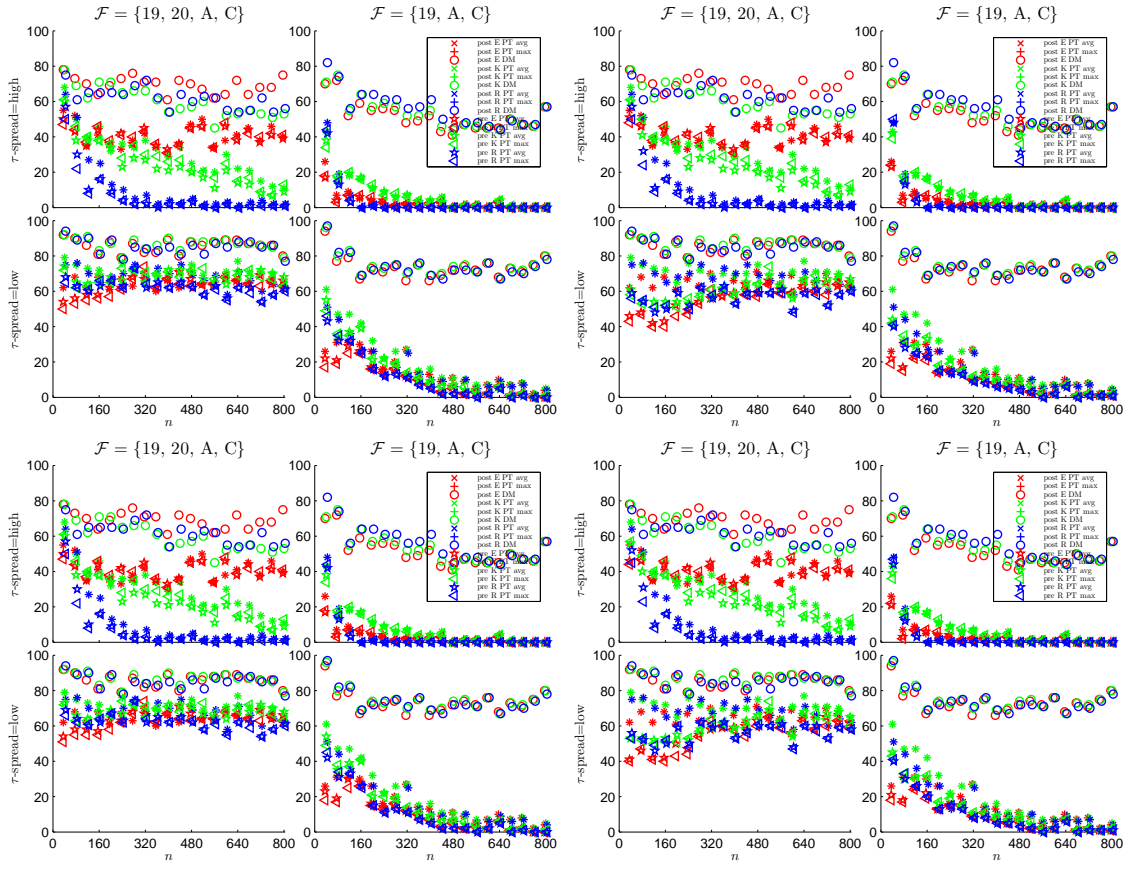

Figure 18: Rejection rate \*\*\* d=10 \*\*\* pessimistic

## 2 The $\mathcal{F}$ -unknown scenario

Here, for each evaluation criterion (except the false families ratio) and  $d \in \{5, 10\}$ , one figure containing the results corresponding to both attitudes (the optimistic case is at the left-hand side and the pessimistic case at the right-hand side) is shown. Each figure is designed in the same way as in the main work, i.e., the results for a given evaluation criterion is shown only for the Re-est=KTauAvg and #Forks=unknown estimators. Also note that the optimistic case is not shown for the rejection rate.

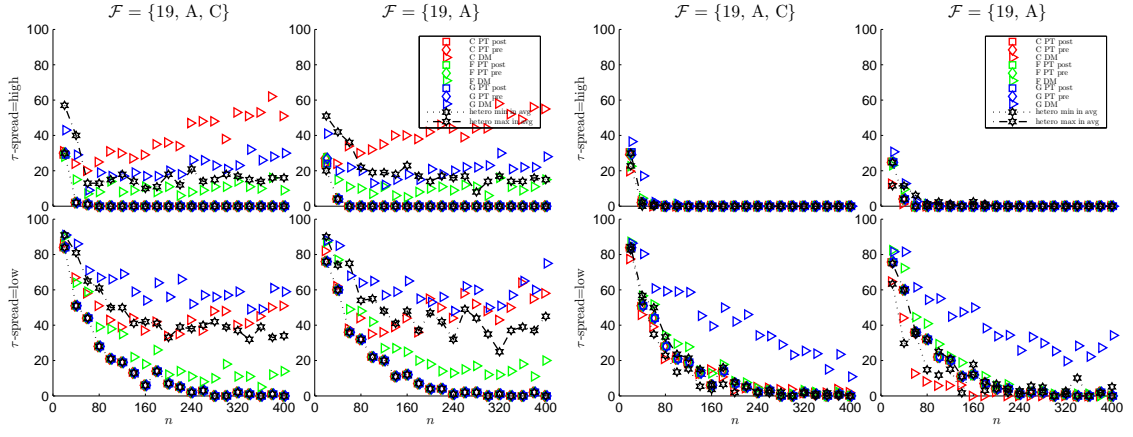

Figure 19: False structure ratio (in %) \*\*\* d=5

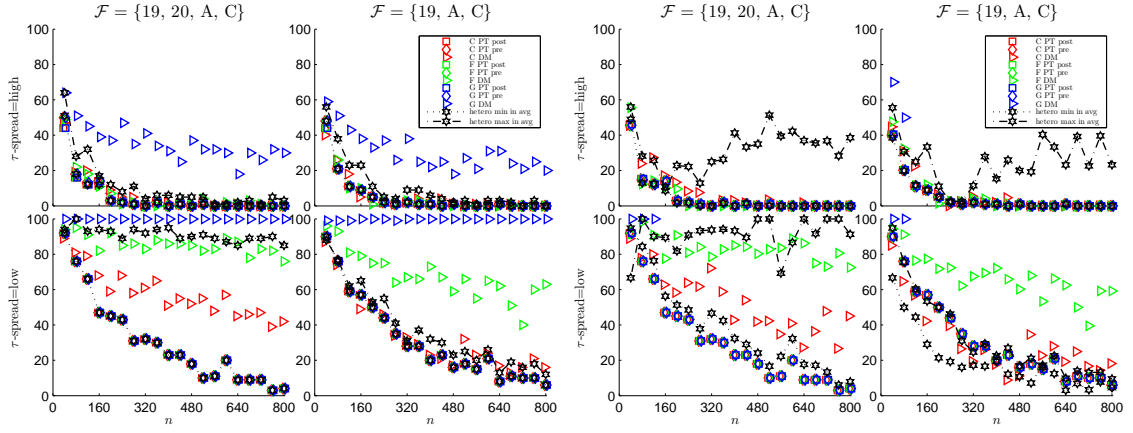

Figure 20: False structure ratio (in %) \*\*\* d=10

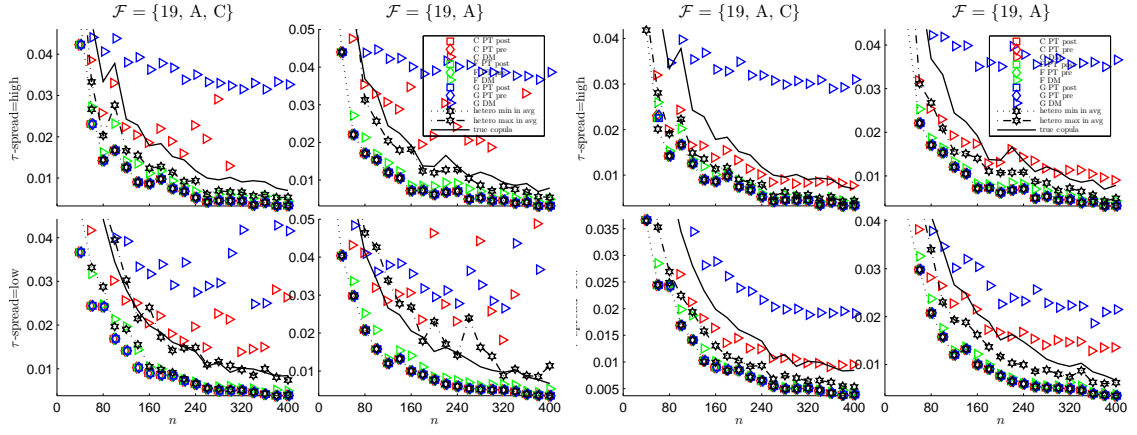

Figure 21: Tau distance median \*\*\* d=5

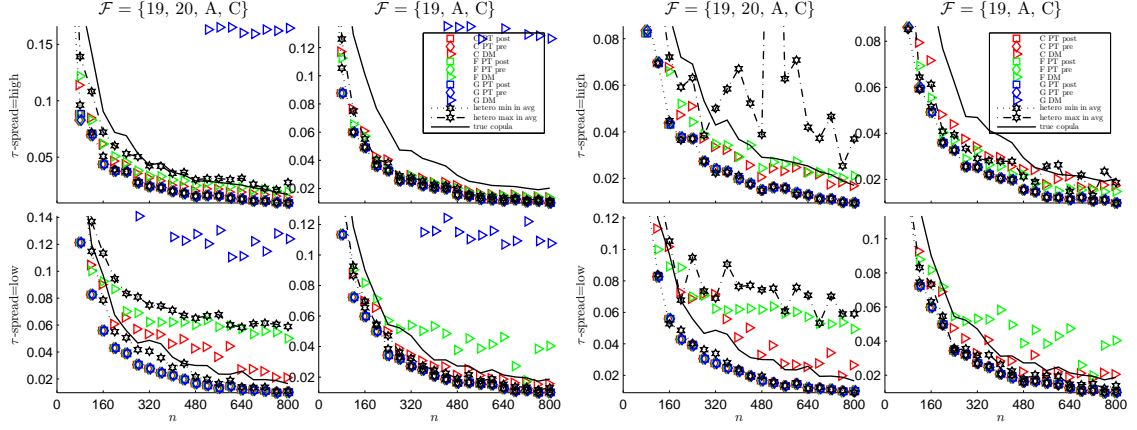

Figure 22: Tau distance median \*\*\* d=10

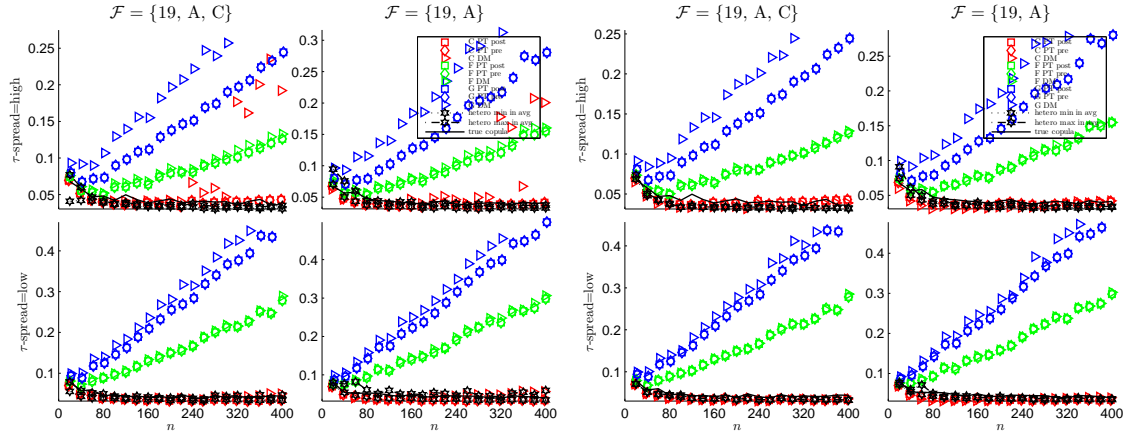

Figure 23: GoF median \*\*\* d=5

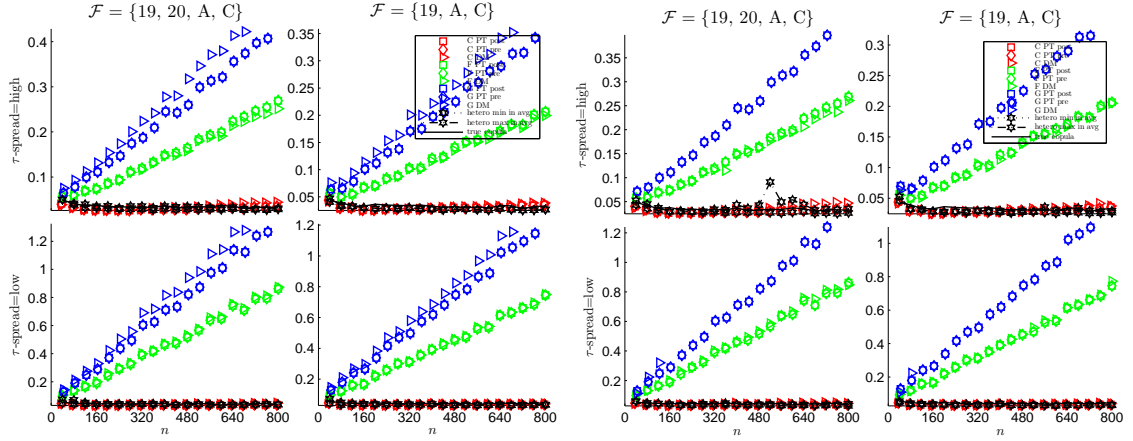

Figure 24: GoF median \*\*\* d=10

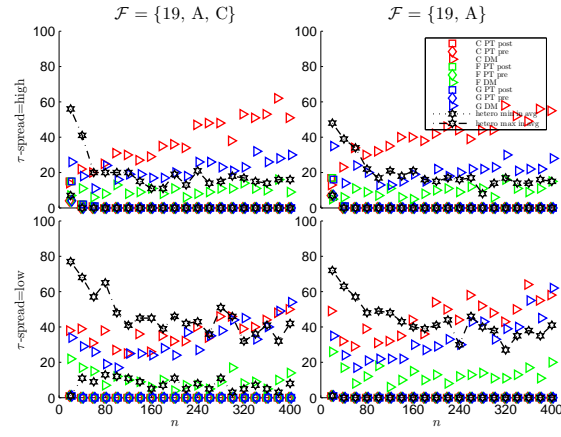

Figure 25: Rejection rate \*\*\* d=5

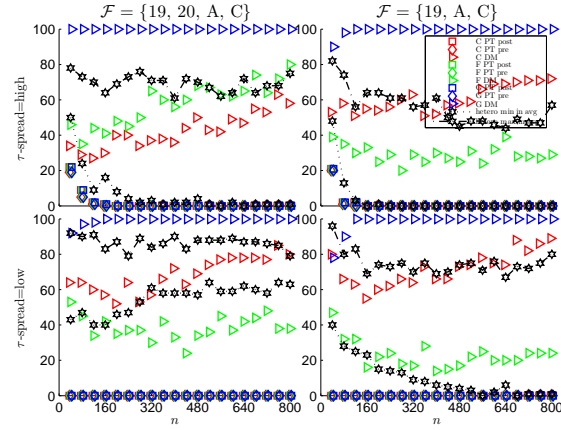

Figure 26: Rejection rate \*\*\* d=10
